# Supplementary material for: Scratch that! An Evolution-based Adversarial Attack against Neural Networks
Source: arXiv:1912.02316 source file (2020-08-06)
Supplement: Supplementary file 1 [file 6_appendix.tex]

\section{Appendix}
